# Supplementary material for: Intrinsic Motivation Driven Intuitive Physics Learning using Deep Reinforcement Learning with Intrinsic Reward Normalization
Source: arXiv:1907.03116 source file (2019-07-06)
Supplement: Supplementary file 1 [file 8.appendix.tex]

% \newcommand{\imscale}{0.125}
% Here we provide qualitative results from 6-object scene. Videos of our results are available here: https://youtu.be/4UP49o5cWbs. We test our agent in single focus object scenes and multiple focus object scenes. Each object is indexed from 0 to 5 where 0 is the object on the bottom left, 1 is the object next to object 0 on the same row, and 5 is the object on the top right. 

% \subsection*{Single Focus Object Results}

% \begin{figure*}[hbt!]
% \begin{center}
% \includegraphics[scale=\imscale]{results/nbObjects6/img_seq_0/image_0.png}
% \includegraphics[scale=\imscale]{results/nbObjects6/img_seq_0/image_1.png}
% \includegraphics[scale=\imscale]{results/nbObjects6/img_seq_0/image_2.png}
% \includegraphics[scale=\imscale]{results/nbObjects6/img_seq_0/image_3.png}
% \includegraphics[scale=\imscale]{results/nbObjects6/img_seq_0/image_4.png}
% \includegraphics[scale=\imscale]{results/nbObjects6/img_seq_0/image_5.png}
% \includegraphics[scale=\imscale]{results/nbObjects6/img_seq_0/image_6.png}
% \includegraphics[scale=\imscale]{results/nbObjects6/img_seq_0/image_7.png}
% \includegraphics[scale=\imscale]{results/nbObjects6/img_seq_0/image_8.png}
% \includegraphics[scale=\imscale]{results/nbObjects6/img_seq_0/image_9.png}
% \includegraphics[scale=\imscale]{results/nbObjects6/img_seq_0/image_10.png}
% \includegraphics[scale=\imscale]{results/nbObjects6/img_seq_0/image_11.png}
% \includegraphics[scale=\imscale]{results/nbObjects6/img_seq_0/image_12.png}
% \includegraphics[scale=\imscale]{results/nbObjects6/img_seq_0/image_13.png}
% \includegraphics[scale=\imscale]{results/nbObjects6/img_seq_0/image_14.png}
% \includegraphics[scale=\imscale]{results/nbObjects6/img_seq_0/image_15.png}
% \includegraphics[scale=\imscale]{results/nbObjects6/img_seq_0/image_16.png}
% \includegraphics[scale=\imscale]{results/nbObjects6/img_seq_0/image_17.png}
% \includegraphics[scale=\imscale]{results/nbObjects6/img_seq_0/image_18.png}
% \includegraphics[scale=\imscale]{results/nbObjects6/img_seq_0/image_19.png}
% \caption{Object 0 applied with normalized force (1,0,0).}
% \label{single_fobj_result_1}
% \end{center}
% \end{figure*}

% \begin{figure*}[hbt!]
% \begin{center}
% \includegraphics[scale=\imscale]{results/nbObjects6/img_seq_2/image_76.png}
% \includegraphics[scale=\imscale]{results/nbObjects6/img_seq_2/image_77.png}
% \includegraphics[scale=\imscale]{results/nbObjects6/img_seq_2/image_78.png}
% \includegraphics[scale=\imscale]{results/nbObjects6/img_seq_2/image_79.png}
% \includegraphics[scale=\imscale]{results/nbObjects6/img_seq_2/image_80.png}
% \includegraphics[scale=\imscale]{results/nbObjects6/img_seq_2/image_81.png}
% \includegraphics[scale=\imscale]{results/nbObjects6/img_seq_2/image_82.png}
% \includegraphics[scale=\imscale]{results/nbObjects6/img_seq_2/image_83.png}
% \includegraphics[scale=\imscale]{results/nbObjects6/img_seq_2/image_84.png}
% \includegraphics[scale=\imscale]{results/nbObjects6/img_seq_2/image_85.png}
% \includegraphics[scale=\imscale]{results/nbObjects6/img_seq_2/image_86.png}
% \includegraphics[scale=\imscale]{results/nbObjects6/img_seq_2/image_88.png}
% \includegraphics[scale=\imscale]{results/nbObjects6/img_seq_2/image_89.png}
% \includegraphics[scale=\imscale]{results/nbObjects6/img_seq_2/image_90.png}
% \includegraphics[scale=\imscale]{results/nbObjects6/img_seq_2/image_91.png}
% \includegraphics[scale=\imscale]{results/nbObjects6/img_seq_2/image_92.png}
% \includegraphics[scale=\imscale]{results/nbObjects6/img_seq_2/image_93.png}
% \includegraphics[scale=\imscale]{results/nbObjects6/img_seq_2/image_94.png}
% \includegraphics[scale=\imscale]{results/nbObjects6/img_seq_2/image_94.png}
% \includegraphics[scale=\imscale]{results/nbObjects6/img_seq_2/image_94.png}
% \caption{Object 1 applied with normalized force (1,0,0).}
% \label{single_fobj_result_2}
% \end{center}
% \end{figure*}

 

% \begin{figure*}[hbt!]
% \begin{center}
% \includegraphics[scale=\imscale]{results/nbObjects6/img_seq_1/image_20.png}
% \includegraphics[scale=\imscale]{results/nbObjects6/img_seq_1/image_21.png}
% \includegraphics[scale=\imscale]{results/nbObjects6/img_seq_1/image_22.png}
% \includegraphics[scale=\imscale]{results/nbObjects6/img_seq_1/image_23.png}
% \includegraphics[scale=\imscale]{results/nbObjects6/img_seq_1/image_24.png}
% \includegraphics[scale=\imscale]{results/nbObjects6/img_seq_1/image_25.png}
% \includegraphics[scale=\imscale]{results/nbObjects6/img_seq_1/image_26.png}
% \includegraphics[scale=\imscale]{results/nbObjects6/img_seq_1/image_27.png}
% \includegraphics[scale=\imscale]{results/nbObjects6/img_seq_1/image_28.png}
% \includegraphics[scale=\imscale]{results/nbObjects6/img_seq_1/image_29.png}
% \includegraphics[scale=\imscale]{results/nbObjects6/img_seq_1/image_30.png}
% \includegraphics[scale=\imscale]{results/nbObjects6/img_seq_1/image_31.png}
% \includegraphics[scale=\imscale]{results/nbObjects6/img_seq_1/image_32.png}
% \includegraphics[scale=\imscale]{results/nbObjects6/img_seq_1/image_33.png}
% \includegraphics[scale=\imscale]{results/nbObjects6/img_seq_1/image_34.png}
% \includegraphics[scale=\imscale]{results/nbObjects6/img_seq_1/image_35.png}
% \includegraphics[scale=\imscale]{results/nbObjects6/img_seq_1/image_36.png}
% \includegraphics[scale=\imscale]{results/nbObjects6/img_seq_1/image_37.png}
% \includegraphics[scale=\imscale]{results/nbObjects6/img_seq_1/image_38.png}
% \includegraphics[scale=\imscale]{results/nbObjects6/img_seq_1/image_39.png}
% \includegraphics[scale=\imscale]{results/nbObjects6/img_seq_1/image_40.png}
% \includegraphics[scale=\imscale]{results/nbObjects6/img_seq_1/image_41.png}
% \includegraphics[scale=\imscale]{results/nbObjects6/img_seq_1/image_42.png}
% \includegraphics[scale=\imscale]{results/nbObjects6/img_seq_1/image_43.png}
% \includegraphics[scale=\imscale]{results/nbObjects6/img_seq_1/image_44.png}
% \includegraphics[scale=\imscale]{results/nbObjects6/img_seq_1/image_45.png}
% \includegraphics[scale=\imscale]{results/nbObjects6/img_seq_1/image_46.png}
% \includegraphics[scale=\imscale]{results/nbObjects6/img_seq_1/image_47.png}
% \includegraphics[scale=\imscale]{results/nbObjects6/img_seq_1/image_48.png}
% \includegraphics[scale=\imscale]{results/nbObjects6/img_seq_1/image_49.png}
% \includegraphics[scale=\imscale]{results/nbObjects6/img_seq_1/image_50.png}
% \includegraphics[scale=\imscale]{results/nbObjects6/img_seq_1/image_51.png}
% \includegraphics[scale=\imscale]{results/nbObjects6/img_seq_1/image_52.png}
% \includegraphics[scale=\imscale]{results/nbObjects6/img_seq_1/image_53.png}
% \includegraphics[scale=\imscale]{results/nbObjects6/img_seq_1/image_54.png}
% \includegraphics[scale=\imscale]{results/nbObjects6/img_seq_1/image_55.png}
% \includegraphics[scale=\imscale]{results/nbObjects6/img_seq_1/image_56.png}
% \includegraphics[scale=\imscale]{results/nbObjects6/img_seq_1/image_57.png}
% \includegraphics[scale=\imscale]{results/nbObjects6/img_seq_1/image_58.png}
% \includegraphics[scale=\imscale]{results/nbObjects6/img_seq_1/image_59.png}
% \includegraphics[scale=\imscale]{results/nbObjects6/img_seq_1/image_60.png}
% \includegraphics[scale=\imscale]{results/nbObjects6/img_seq_1/image_61.png}
% \includegraphics[scale=\imscale]{results/nbObjects6/img_seq_1/image_62.png}
% \includegraphics[scale=\imscale]{results/nbObjects6/img_seq_1/image_63.png}
% \includegraphics[scale=\imscale]{results/nbObjects6/img_seq_1/image_64.png}
% \includegraphics[scale=\imscale]{results/nbObjects6/img_seq_1/image_65.png}
% \includegraphics[scale=\imscale]{results/nbObjects6/img_seq_1/image_66.png}
% \includegraphics[scale=\imscale]{results/nbObjects6/img_seq_1/image_67.png}
% \includegraphics[scale=\imscale]{results/nbObjects6/img_seq_1/image_68.png}
% \includegraphics[scale=\imscale]{results/nbObjects6/img_seq_1/image_69.png}
% \caption{Object 1 applied with normalized force (1,1,0).}
% \label{single_fobj_result_3}
% \end{center}
% \end{figure*}


% \newpage
% \subsection*{Multiple Focus Objects Results}

% \begin{figure*}[hbt!]
% \begin{center}
% \includegraphics[scale=\imscale]{results/nbObjects6/img_seq_4/image_133.png}
% \includegraphics[scale=\imscale]{results/nbObjects6/img_seq_4/image_134.png}
% \includegraphics[scale=\imscale]{results/nbObjects6/img_seq_4/image_135.png}
% \includegraphics[scale=\imscale]{results/nbObjects6/img_seq_4/image_136.png}
% \includegraphics[scale=\imscale]{results/nbObjects6/img_seq_4/image_137.png}
% \includegraphics[scale=\imscale]{results/nbObjects6/img_seq_4/image_138.png}
% \includegraphics[scale=\imscale]{results/nbObjects6/img_seq_4/image_139.png}
% \includegraphics[scale=\imscale]{results/nbObjects6/img_seq_4/image_140.png}
% \includegraphics[scale=\imscale]{results/nbObjects6/img_seq_4/image_141.png}
% \includegraphics[scale=\imscale]{results/nbObjects6/img_seq_4/image_142.png}
% \includegraphics[scale=\imscale]{results/nbObjects6/img_seq_4/image_143.png}
% \includegraphics[scale=\imscale]{results/nbObjects6/img_seq_4/image_144.png}
% \includegraphics[scale=\imscale]{results/nbObjects6/img_seq_4/image_145.png}
% \includegraphics[scale=\imscale]{results/nbObjects6/img_seq_4/image_146.png}
% \includegraphics[scale=\imscale]{results/nbObjects6/img_seq_4/image_147.png}
% \includegraphics[scale=\imscale]{results/nbObjects6/img_seq_4/image_148.png}
% \includegraphics[scale=\imscale]{results/nbObjects6/img_seq_4/image_149.png}
% \includegraphics[scale=\imscale]{results/nbObjects6/img_seq_4/image_150.png}
% \includegraphics[scale=\imscale]{results/nbObjects6/img_seq_4/image_151.png}
% \includegraphics[scale=\imscale]{results/nbObjects6/img_seq_4/image_152.png}
% \includegraphics[scale=\imscale]{results/nbObjects6/img_seq_4/image_153.png}
% \includegraphics[scale=\imscale]{results/nbObjects6/img_seq_4/image_154.png}
% \includegraphics[scale=\imscale]{results/nbObjects6/img_seq_4/image_155.png}
% \includegraphics[scale=\imscale]{results/nbObjects6/img_seq_4/image_156.png}
% \includegraphics[scale=\imscale]{results/nbObjects6/img_seq_4/image_157.png}
% \includegraphics[scale=\imscale]{results/nbObjects6/img_seq_4/image_158.png}
% \includegraphics[scale=\imscale]{results/nbObjects6/img_seq_4/image_159.png}
% \includegraphics[scale=\imscale]{results/nbObjects6/img_seq_4/image_160.png}
% \includegraphics[scale=\imscale]{results/nbObjects6/img_seq_4/image_161.png}
% \includegraphics[scale=\imscale]{results/nbObjects6/img_seq_4/image_162.png}
% \includegraphics[scale=\imscale]{results/nbObjects6/img_seq_4/image_163.png}
% \includegraphics[scale=\imscale]{results/nbObjects6/img_seq_4/image_164.png}
% \includegraphics[scale=\imscale]{results/nbObjects6/img_seq_4/image_165.png}
% \includegraphics[scale=\imscale]{results/nbObjects6/img_seq_4/image_166.png}
% \includegraphics[scale=\imscale]{results/nbObjects6/img_seq_4/image_167.png}
% \includegraphics[scale=\imscale]{results/nbObjects6/img_seq_4/image_168.png}
% \includegraphics[scale=\imscale]{results/nbObjects6/img_seq_4/image_169.png}
% \includegraphics[scale=\imscale]{results/nbObjects6/img_seq_4/image_170.png}
% \includegraphics[scale=\imscale]{results/nbObjects6/img_seq_4/image_171.png}
% \includegraphics[scale=\imscale]{results/nbObjects6/img_seq_4/image_172.png}
% \includegraphics[scale=\imscale]{results/nbObjects6/img_seq_4/image_173.png}
% \includegraphics[scale=\imscale]{results/nbObjects6/img_seq_4/image_174.png}
% \includegraphics[scale=\imscale]{results/nbObjects6/img_seq_4/image_175.png}
% \includegraphics[scale=\imscale]{results/nbObjects6/img_seq_4/image_176.png}
% \includegraphics[scale=\imscale]{results/nbObjects6/img_seq_4/image_177.png}
% \includegraphics[scale=\imscale]{results/nbObjects6/img_seq_4/image_178.png}
% \includegraphics[scale=\imscale]{results/nbObjects6/img_seq_4/image_179.png}
% \includegraphics[scale=\imscale]{results/nbObjects6/img_seq_4/image_180.png}
% \includegraphics[scale=\imscale]{results/nbObjects6/img_seq_4/image_181.png}
% \includegraphics[scale=\imscale]{results/nbObjects6/img_seq_4/image_182.png}
% \includegraphics[scale=\imscale]{results/nbObjects6/img_seq_4/image_183.png}
% \includegraphics[scale=\imscale]{results/nbObjects6/img_seq_4/image_184.png}
% \includegraphics[scale=\imscale]{results/nbObjects6/img_seq_4/image_185.png}
% \includegraphics[scale=\imscale]{results/nbObjects6/img_seq_4/image_186.png}
% \includegraphics[scale=\imscale]{results/nbObjects6/img_seq_4/image_187.png}
% \includegraphics[scale=\imscale]{results/nbObjects6/img_seq_4/image_188.png}
% \includegraphics[scale=\imscale]{results/nbObjects6/img_seq_4/image_189.png}
% \includegraphics[scale=\imscale]{results/nbObjects6/img_seq_4/image_190.png}
% \includegraphics[scale=\imscale]{results/nbObjects6/img_seq_4/image_191.png}
% \includegraphics[scale=\imscale]{results/nbObjects6/img_seq_4/image_192.png}
% \caption{All objects applied with normalized force (0,0,1).}
% \label{multiple_fobj_result_1}
% \end{center}
% \end{figure*}


% \begin{figure*}[hbt!]
% \begin{center}
% \includegraphics[scale=\imscale]{results/nbObjects6/img_seq_17/image_1075.png}
% \includegraphics[scale=\imscale]{results/nbObjects6/img_seq_17/image_1076.png}
% \includegraphics[scale=\imscale]{results/nbObjects6/img_seq_17/image_1077.png}
% \includegraphics[scale=\imscale]{results/nbObjects6/img_seq_17/image_1078.png}
% \includegraphics[scale=\imscale]{results/nbObjects6/img_seq_17/image_1079.png}
% \includegraphics[scale=\imscale]{results/nbObjects6/img_seq_17/image_1080.png}
% \includegraphics[scale=\imscale]{results/nbObjects6/img_seq_17/image_1081.png}
% \includegraphics[scale=\imscale]{results/nbObjects6/img_seq_17/image_1082.png}
% \includegraphics[scale=\imscale]{results/nbObjects6/img_seq_17/image_1083.png}
% \includegraphics[scale=\imscale]{results/nbObjects6/img_seq_17/image_1084.png}
% \includegraphics[scale=\imscale]{results/nbObjects6/img_seq_17/image_1085.png}
% \includegraphics[scale=\imscale]{results/nbObjects6/img_seq_17/image_1086.png}
% \includegraphics[scale=\imscale]{results/nbObjects6/img_seq_17/image_1087.png}
% \includegraphics[scale=\imscale]{results/nbObjects6/img_seq_17/image_1088.png}
% \includegraphics[scale=\imscale]{results/nbObjects6/img_seq_17/image_1089.png}
% \includegraphics[scale=\imscale]{results/nbObjects6/img_seq_17/image_1090.png}
% \includegraphics[scale=\imscale]{results/nbObjects6/img_seq_17/image_1091.png}
% \includegraphics[scale=\imscale]{results/nbObjects6/img_seq_17/image_1092.png}
% \includegraphics[scale=\imscale]{results/nbObjects6/img_seq_17/image_1093.png}
% \includegraphics[scale=\imscale]{results/nbObjects6/img_seq_17/image_1094.png}
% \includegraphics[scale=\imscale]{results/nbObjects6/img_seq_17/image_1095.png}
% \includegraphics[scale=\imscale]{results/nbObjects6/img_seq_17/image_1096.png}
% \includegraphics[scale=\imscale]{results/nbObjects6/img_seq_17/image_1097.png}
% \includegraphics[scale=\imscale]{results/nbObjects6/img_seq_17/image_1098.png}
% \includegraphics[scale=\imscale]{results/nbObjects6/img_seq_17/image_1099.png}
% \includegraphics[scale=\imscale]{results/nbObjects6/img_seq_17/image_1100.png}
% \includegraphics[scale=\imscale]{results/nbObjects6/img_seq_17/image_1101.png}
% \includegraphics[scale=\imscale]{results/nbObjects6/img_seq_17/image_1102.png}
% \includegraphics[scale=\imscale]{results/nbObjects6/img_seq_17/image_1103.png}
% \includegraphics[scale=\imscale]{results/nbObjects6/img_seq_17/image_1104.png}
% \includegraphics[scale=\imscale]{results/nbObjects6/img_seq_17/image_1105.png}
% \includegraphics[scale=\imscale]{results/nbObjects6/img_seq_17/image_1106.png}
% \includegraphics[scale=\imscale]{results/nbObjects6/img_seq_17/image_1107.png}
% \includegraphics[scale=\imscale]{results/nbObjects6/img_seq_17/image_1108.png}
% \includegraphics[scale=\imscale]{results/nbObjects6/img_seq_17/image_1109.png}
% \includegraphics[scale=\imscale]{results/nbObjects6/img_seq_17/image_1110.png}
% \includegraphics[scale=\imscale]{results/nbObjects6/img_seq_17/image_1111.png}
% \includegraphics[scale=\imscale]{results/nbObjects6/img_seq_17/image_1112.png}
% \includegraphics[scale=\imscale]{results/nbObjects6/img_seq_17/image_1113.png}
% \includegraphics[scale=\imscale]{results/nbObjects6/img_seq_17/image_1114.png}
% \caption{Object 3 and object 5 applied with normalized forces (1,-1,0), and (-1,-1,0).}
% \label{multiple_fobj_result_2}
% \end{center}
% \end{figure*}


% \begin{figure*}[hbt!]
% \begin{center}
% \includegraphics[scale=\imscale]{results/nbObjects6/img_seq_10/image_440.png}
% \includegraphics[scale=\imscale]{results/nbObjects6/img_seq_10/image_441.png}
% \includegraphics[scale=\imscale]{results/nbObjects6/img_seq_10/image_442.png}
% \includegraphics[scale=\imscale]{results/nbObjects6/img_seq_10/image_443.png}
% \includegraphics[scale=\imscale]{results/nbObjects6/img_seq_10/image_444.png}
% \includegraphics[scale=\imscale]{results/nbObjects6/img_seq_10/image_445.png}
% \includegraphics[scale=\imscale]{results/nbObjects6/img_seq_10/image_446.png}
% \includegraphics[scale=\imscale]{results/nbObjects6/img_seq_10/image_447.png}
% \includegraphics[scale=\imscale]{results/nbObjects6/img_seq_10/image_448.png}
% \includegraphics[scale=\imscale]{results/nbObjects6/img_seq_10/image_449.png}
% \includegraphics[scale=\imscale]{results/nbObjects6/img_seq_10/image_450.png}
% \includegraphics[scale=\imscale]{results/nbObjects6/img_seq_10/image_451.png}
% \includegraphics[scale=\imscale]{results/nbObjects6/img_seq_10/image_452.png}
% \includegraphics[scale=\imscale]{results/nbObjects6/img_seq_10/image_453.png}
% \includegraphics[scale=\imscale]{results/nbObjects6/img_seq_10/image_454.png}
% \includegraphics[scale=\imscale]{results/nbObjects6/img_seq_10/image_455.png}
% \includegraphics[scale=\imscale]{results/nbObjects6/img_seq_10/image_456.png}
% \includegraphics[scale=\imscale]{results/nbObjects6/img_seq_10/image_457.png}
% \includegraphics[scale=\imscale]{results/nbObjects6/img_seq_10/image_458.png}
% \includegraphics[scale=\imscale]{results/nbObjects6/img_seq_10/image_459.png}
% \includegraphics[scale=\imscale]{results/nbObjects6/img_seq_10/image_460.png}
% \includegraphics[scale=\imscale]{results/nbObjects6/img_seq_10/image_461.png}
% \includegraphics[scale=\imscale]{results/nbObjects6/img_seq_10/image_462.png}
% \includegraphics[scale=\imscale]{results/nbObjects6/img_seq_10/image_463.png}
% \includegraphics[scale=\imscale]{results/nbObjects6/img_seq_10/image_464.png}
% \includegraphics[scale=\imscale]{results/nbObjects6/img_seq_10/image_465.png}
% \includegraphics[scale=\imscale]{results/nbObjects6/img_seq_10/image_466.png}
% \includegraphics[scale=\imscale]{results/nbObjects6/img_seq_10/image_467.png}
% \includegraphics[scale=\imscale]{results/nbObjects6/img_seq_10/image_468.png}
% \includegraphics[scale=\imscale]{results/nbObjects6/img_seq_10/image_469.png}
% \includegraphics[scale=\imscale]{results/nbObjects6/img_seq_10/image_470.png}
% \includegraphics[scale=\imscale]{results/nbObjects6/img_seq_10/image_471.png}
% \includegraphics[scale=\imscale]{results/nbObjects6/img_seq_10/image_472.png}
% \includegraphics[scale=\imscale]{results/nbObjects6/img_seq_10/image_473.png}
% \includegraphics[scale=\imscale]{results/nbObjects6/img_seq_10/image_474.png}
% \includegraphics[scale=\imscale]{results/nbObjects6/img_seq_10/image_475.png}
% \includegraphics[scale=\imscale]{results/nbObjects6/img_seq_10/image_476.png}
% \includegraphics[scale=\imscale]{results/nbObjects6/img_seq_10/image_477.png}
% \includegraphics[scale=\imscale]{results/nbObjects6/img_seq_10/image_478.png}
% \includegraphics[scale=\imscale]{results/nbObjects6/img_seq_10/image_479.png}
% \includegraphics[scale=\imscale]{results/nbObjects6/img_seq_10/image_480.png}
% \includegraphics[scale=\imscale]{results/nbObjects6/img_seq_10/image_481.png}
% \includegraphics[scale=\imscale]{results/nbObjects6/img_seq_10/image_482.png}
% \includegraphics[scale=\imscale]{results/nbObjects6/img_seq_10/image_483.png}
% \includegraphics[scale=\imscale]{results/nbObjects6/img_seq_10/image_484.png}
% \includegraphics[scale=\imscale]{results/nbObjects6/img_seq_10/image_485.png}
% \includegraphics[scale=\imscale]{results/nbObjects6/img_seq_10/image_486.png}
% \includegraphics[scale=\imscale]{results/nbObjects6/img_seq_10/image_487.png}
% \includegraphics[scale=\imscale]{results/nbObjects6/img_seq_10/image_488.png}
% \includegraphics[scale=\imscale]{results/nbObjects6/img_seq_10/image_489.png}
% \caption{Object 3, object 4 and object 5 applied with normalized force (0,1,0).}
% \label{multiple_fobj_result_3}
% \end{center}
% \end{figure*}



% \begin{figure*}[hbt!]
% \begin{center}
% \includegraphics[scale=\imscale]{results/nbObjects6/img_seq_16/image_975.png}
% \includegraphics[scale=\imscale]{results/nbObjects6/img_seq_16/image_976.png}
% \includegraphics[scale=\imscale]{results/nbObjects6/img_seq_16/image_977.png}
% \includegraphics[scale=\imscale]{results/nbObjects6/img_seq_16/image_978.png}
% \includegraphics[scale=\imscale]{results/nbObjects6/img_seq_16/image_979.png}
% \includegraphics[scale=\imscale]{results/nbObjects6/img_seq_16/image_980.png}
% \includegraphics[scale=\imscale]{results/nbObjects6/img_seq_16/image_981.png}
% \includegraphics[scale=\imscale]{results/nbObjects6/img_seq_16/image_982.png}
% \includegraphics[scale=\imscale]{results/nbObjects6/img_seq_16/image_983.png}
% \includegraphics[scale=\imscale]{results/nbObjects6/img_seq_16/image_984.png}
% \includegraphics[scale=\imscale]{results/nbObjects6/img_seq_16/image_985.png}
% \includegraphics[scale=\imscale]{results/nbObjects6/img_seq_16/image_986.png}
% \includegraphics[scale=\imscale]{results/nbObjects6/img_seq_16/image_987.png}
% \includegraphics[scale=\imscale]{results/nbObjects6/img_seq_16/image_988.png}
% \includegraphics[scale=\imscale]{results/nbObjects6/img_seq_16/image_989.png}
% \includegraphics[scale=\imscale]{results/nbObjects6/img_seq_16/image_990.png}
% \includegraphics[scale=\imscale]{results/nbObjects6/img_seq_16/image_991.png}
% \includegraphics[scale=\imscale]{results/nbObjects6/img_seq_16/image_992.png}
% \includegraphics[scale=\imscale]{results/nbObjects6/img_seq_16/image_993.png}
% \includegraphics[scale=\imscale]{results/nbObjects6/img_seq_16/image_994.png}
% \includegraphics[scale=\imscale]{results/nbObjects6/img_seq_16/image_995.png}
% \includegraphics[scale=\imscale]{results/nbObjects6/img_seq_16/image_996.png}
% \includegraphics[scale=\imscale]{results/nbObjects6/img_seq_16/image_997.png}
% \includegraphics[scale=\imscale]{results/nbObjects6/img_seq_16/image_998.png}
% \includegraphics[scale=\imscale]{results/nbObjects6/img_seq_16/image_999.png}
% \includegraphics[scale=\imscale]{results/nbObjects6/img_seq_16/image_1000.png}
% \includegraphics[scale=\imscale]{results/nbObjects6/img_seq_16/image_1001.png}
% \includegraphics[scale=\imscale]{results/nbObjects6/img_seq_16/image_1002.png}
% \includegraphics[scale=\imscale]{results/nbObjects6/img_seq_16/image_1003.png}
% \includegraphics[scale=\imscale]{results/nbObjects6/img_seq_16/image_1004.png}
% \includegraphics[scale=\imscale]{results/nbObjects6/img_seq_16/image_1005.png}
% \includegraphics[scale=\imscale]{results/nbObjects6/img_seq_16/image_1006.png}
% \includegraphics[scale=\imscale]{results/nbObjects6/img_seq_16/image_1007.png}
% \includegraphics[scale=\imscale]{results/nbObjects6/img_seq_16/image_1008.png}
% \includegraphics[scale=\imscale]{results/nbObjects6/img_seq_16/image_1009.png}
% \includegraphics[scale=\imscale]{results/nbObjects6/img_seq_16/image_1010.png}
% \includegraphics[scale=\imscale]{results/nbObjects6/img_seq_16/image_1011.png}
% \includegraphics[scale=\imscale]{results/nbObjects6/img_seq_16/image_1012.png}
% \includegraphics[scale=\imscale]{results/nbObjects6/img_seq_16/image_1013.png}
% \includegraphics[scale=\imscale]{results/nbObjects6/img_seq_16/image_1014.png}
% \includegraphics[scale=\imscale]{results/nbObjects6/img_seq_16/image_1015.png}
% \includegraphics[scale=\imscale]{results/nbObjects6/img_seq_16/image_1016.png}
% \includegraphics[scale=\imscale]{results/nbObjects6/img_seq_16/image_1017.png}
% \includegraphics[scale=\imscale]{results/nbObjects6/img_seq_16/image_1018.png}
% \includegraphics[scale=\imscale]{results/nbObjects6/img_seq_16/image_1019.png}
% \includegraphics[scale=\imscale]{results/nbObjects6/img_seq_16/image_1020.png}
% \includegraphics[scale=\imscale]{results/nbObjects6/img_seq_16/image_1021.png}
% \includegraphics[scale=\imscale]{results/nbObjects6/img_seq_16/image_1022.png}
% \includegraphics[scale=\imscale]{results/nbObjects6/img_seq_16/image_1023.png}
% \includegraphics[scale=\imscale]{results/nbObjects6/img_seq_16/image_1024.png}
% \includegraphics[scale=\imscale]{results/nbObjects6/img_seq_16/image_1025.png}
% \includegraphics[scale=\imscale]{results/nbObjects6/img_seq_16/image_1026.png}
% \includegraphics[scale=\imscale]{results/nbObjects6/img_seq_16/image_1027.png}
% \includegraphics[scale=\imscale]{results/nbObjects6/img_seq_16/image_1028.png}
% \includegraphics[scale=\imscale]{results/nbObjects6/img_seq_16/image_1029.png}
% \includegraphics[scale=\imscale]{results/nbObjects6/img_seq_16/image_1030.png}
% \includegraphics[scale=\imscale]{results/nbObjects6/img_seq_16/image_1031.png}
% \includegraphics[scale=\imscale]{results/nbObjects6/img_seq_16/image_1032.png}
% \includegraphics[scale=\imscale]{results/nbObjects6/img_seq_16/image_1033.png}
% \includegraphics[scale=\imscale]{results/nbObjects6/img_seq_16/image_1034.png}
% \caption{Object 0 and object 2 applied with normalized force (1,1,0) and (-1,1,0).}
% \label{multiple_fobj_result_4}
% \end{center}
% \end{figure*}
